# Supplementary material for: RefAerial: A Benchmark and Approach for Referring Detection in Aerial Images
Source: arXiv:2604.20543 source file (2026-04-23)
Supplement: Supplementary file 1 [file X_suppl.tex]

\maketitlesupplementary

In this supplementary material, (1) we firstly compare the annotation efficiency between human annotators and the REA-Engine. (2) we then introduce some details and samples about the RefAerial dataset. (3) we further present additional Analysis of the RefAerial Dataset.  (4) we finally introduce more details of the MoG algorithm and its multi-scale attention mechanism.

\section{Comparison between  the REA-Engine and Human Annotators}
Figure \ref{fig:14} compares the annotation performance between human annotators and the proposed REA-Engine within the human-in-the-loop pipeline.\hspace{0.5em}In terms of efficiency, the REA-Engine reduces the annotation time from 5.0~mins/image (human) to 1.0~mins/image, achieving an approximate \textbf{5$\times$} improvement in annotation speed. Despite requiring less human effort, the engine generates slightly longer referring expressions (12.4 vs.\ 8.5 words), suggesting that it naturally incorporates more contextual cues. More importantly, the REA-Engine achieves a substantially higher annotation completeness of 85.0\% compared with 60.0\% for human annotators, indicating its ability to capture richer and more comprehensive target attributes and spatial relations. These results demonstrate that the REA-Engine not only effectively improves annotation efficiency but also significantly enhances annotation quality.

\begin{figure}[h]  % 使用figure环境可以为图片添加标题，并自动管理图片位置
    \centering
    \includegraphics[page=1, width=0.95\linewidth, keepaspectratio]{CVPR26/author-kit-CVPR2026-v1-latex-/sec/human_vs_rea.pdf} 
    \caption{Performance of the REA-Engine and human annotators.
} 
    %In the RefAerial dataset, words related to spatial positions or directions occur with high frequency and are used to describe the relative positions of objects.}  % 图片标题
    \label{fig:14}  % 可选的标签，便于在文档中引用
\end{figure}

\section{Additional Details of the RefAerial Dataset}
Figure \ref{fig:17} shows representative aerial samples from the RefAerial dataset, covering various scenes such as highway interchanges, urban intersections, residential areas, and school playgrounds.
These images were captured by drones at different flight altitudes (30 m, 90 m, and 150 m) and camera angles (0–90°), under diverse lighting and weather conditions including daytime, nighttime, and overcast skies.
They reflect  rich variation in spatial scales and environmental diversity.
The scenes feature dense targets and numerous distractors, including vehicles, pedestrians, bicycles, and complex spatial layouts, making RefAerial a highly challenging benchmark for referring detection in aerial-view scenarios.

\section{Additional Analysis of the RefAerial Dataset}

Figure \ref{fig:15} presents the top 10 most frequent object categories in the RefAerial dataset. Among them, person and sedan dominate the distribution with significantly higher instance counts than other classes. Tree, electric bike, and road markings appear at medium frequency, reflecting common elements in aerial scenes. Categories such as bicycle, snack stand, SUV, street lamp, and manhole cover occur less frequently but still maintain stable presence. Overall, the distribution highlights the dominance of people, vehicles, and basic environmental elements in aerial imagery.

\begin{figure*}[!ht]
\centering
\includegraphics[width=\linewidth]{CVPR26/author-kit-CVPR2026-v1-latex-/sec/附录.pdf}
\caption{More samples from our RefAerial benchmark for referring detection in aerial images.}
\label{fig:17}
\end{figure*}

\begin{figure}[h]  % 使用figure环境可以为图片添加标题，并自动管理图片位置
    \centering
    \includegraphics[page=1, width=1\linewidth, keepaspectratio]{CVPR26/author-kit-CVPR2026-v1-latex-/sec/top10_categories_times_new_roman_nogrid_tall.pdf} 
    \caption{Top 10 Target Categories in the RefAerial dataset.} 
    %In the RefAerial dataset, words related to spatial positions or directions occur with high frequency and are used to describe the relative positions of objects.}  % 图片标题
    \label{fig:15}  % 可选的标签，便于在文档中引用
\end{figure}

\begin{figure}[h]  % 使用figure环境可以为图片添加标题，并自动管理图片位置
    \centering
    \includegraphics[page=1, width=\linewidth, keepaspectratio]{CVPR26/author-kit-CVPR2026-v1-latex-/sec/sentence_length_times_new_roman.pdf} 
    \caption{Distribution of sentence length in the RefAerial dataset.
}
    \label{fig:16}  % 可选的标签，便于在文档中引用
\end{figure}

Figure~\ref{fig:16} shows the distribution of sentence lengths in the RefAerial dataset. Most expressions contain 10--15 words, while short ($<10$ words) and long ($>15$ words) descriptions appear less frequently. The overall pattern suggests that the dataset favors moderately long referring expressions, providing sufficient detail for grounding tasks.

\section{Additional details of the MoG algorithm}
The Mixture-of-Granularity (MoG) mechanism introduces a structured multi-scale inductive bias into the standard dot-product attention. Conventional attention connects every query to all key positions uniformly, which often results in redundant interactions and limited ability to model hierarchical context. MoG instead employs a set of dilation-controlled branches, each associated with a dilation rate $d_g \in \mathcal{D}$, where a binary mask $M^{(g)}_{i,j}=1$ only when the index distance $|i-j|$ satisfies a modulo constraint with respect to $d_g$. This mask produces a sparsified attention pattern and defines masked logits $\widetilde{A}^{(g)} = A + \log M^{(g)}$, ensuring that infeasible connections contribute exactly zero under softmax. Each branch computes a partial attention output $Y^{(g)} = \mathrm{softmax}(\widetilde{A}^{(g)})V$, capturing contextual cues at its particular granularity. A lightweight gating network then computes mixture weights $\gamma_g$ from a pooled representation of $X$, and the final attention output is obtained via the convex combination $Y = \sum_g \gamma_g\, Y^{(g)}$.

\begin{algorithm*}[t]
\caption{Flowchart of the Mixture-of-Granularity (MoG) Attention}
// \emph{Assume token sequence $X\in\mathbb{R}^{B\times N\times D}$;}\\
// \emph{Assume dilation set $\mathcal{D}=\{d_g\}_{g=1}^{G}$ for $G$ granularities;}\\
 // \emph{Assume projection matrices $W_Q,W_K,W_V\in\mathbb{R}^{D\times D}$;}\\
 // \emph{Assume gating parameters $W_g\in\mathbb{R}^{D\times G}$ and $b_g\in\mathbb{R}^{G}$;}\\
 // \emph{Assume $d_k$ is the head dimension for scaled dot-product attention.}

\KwIn{token sequence $X$, dilation set $\mathcal{D}$}
\KwOut{attended feature $Y$}

\tcp{Step 1: base attention logits}
Compute query / key / value projections: \\
\Indp
$Q \gets XW_Q$; $K \gets XW_K$; $V \gets XW_V$ \\
$A_{b,i,j} \gets \dfrac{Q_{b,i,:}K_{b,j,:}^{\top}}{\sqrt{d_k}}$ \tcp*{scaled dot-product logits}
\Indm

\vspace{0.3em}
\tcp{Step 2: structured sparse attention branches}
$g \gets 1$ \\
\Repeat{$g > G$}{
    $d_g \gets \mathcal{D}[g]$ \tcp*{granularity dilation}

    \tcp{construct binary mask $M^{(g)}$}
    \For{each index pair $(i,j)$}{
        $d \gets |i-j|$ \\
        \uIf{$d \bmod d_g = 0$}{
            $M^{(g)}_{i,j} \gets 1$
        }\Else{
            $M^{(g)}_{i,j} \gets 0$
        }
    }

    \tcp{masked attention for granularity $g$}
    $\widetilde{A}^{(g)}_{b,i,j} \gets A_{b,i,j} + \log M^{(g)}_{i,j}$ \\
    $\alpha^{(g)}_{b,i,j} \gets
        \operatorname{softmax}_{j}
        \big(\widetilde{A}^{(g)}_{b,i,j}\big)$ \\
    $Y^{(g)}_{b,i,:} \gets
        \sum_{j=1}^{N} \alpha^{(g)}_{b,i,j} V_{b,j,:}$ \tcp*{branch output}

    $g \gets g+1$
}

\vspace{0.3em}
\tcp{Step 3: granularity fusion network}
\For{each batch index $b$}{
    $\bar{X}_b \gets \dfrac{1}{N}\sum_{i=1}^{N} X_{b,i,:}$ \tcp*{global pooling}
    $\hat{X}_b \gets \mathrm{LayerNorm}(\bar{X}_b)$ \tcp*{normalization}

    \tcp{gating logits and mixture weights}
    \For{$g \gets 1$ \KwTo $G$}{
        $z_{b,g} \gets (W_g^\top \hat{X}_b + b_g)_g$
    }
    $\gamma_{b,g} \gets \operatorname{softmax}_g(z_{b,g})$ \tcp*{mixture over granularities}
}

\vspace{0.3em}
\tcp{Step 4: final MoG output}
\For{each $(b,i)$}{
    $Y_{b,i,:} \gets \sum_{g=1}^{G} \gamma_{b,g}\, Y^{(g)}_{b,i,:}$
}

\Return{$Y$}

\label{Algo_MoG}
\end{algorithm*}
